# Supplementary material for: Distributed Adaptive Backstepping Control for Vehicular Platoons with Mismatched Disturbances Using Vector String Lyapunov Functions
Source: arXiv:2207.02101 source file (2022-11-29)
Supplement: Supplementary file 1 [file additional.tex]

To determine the corresponding partition in the abstraction's space, i.e. \(\mathbf{D}_{zj}z\geq \mathbf{E}_{zj}\), based on the desired partition in concrete system's space, i.e. \(\mathbf{D}_{j}x\geq \mathbf{E}_{j}\), the following lemma is applied:

\begin{lemma} \cite{??,??}
    Given a polytope \(\mathcal{Z}=\{\mathbf{z}\in\mathbb{R}^m|\mathbf{D}_{zj}\mathbf{z}\geq \mathbf{E}_{zj}\}\), \(\mathbf{P}_i\in\mathbb{R}^{n\times m}\), \(\mathbf{\hat{y}}\in\mathbb{R}^n\), and \(\mathcal{X}_j=\{\mathbf{x}\in\mathbb{R}^n|\mathbf{D}_j\mathbf{x}\geq \mathbf{E}_j\}\), \(j=1,...,r\), the condition \(\mathbf{P}_i\mathcal{Z}+\mathbf{\hat{y}}\subseteq\mathcal{X}_j\) is equivalent to
    \begin{equation}
        \mathbf{\Lambda}_k\mathbf{D}_{zj}=\mathbf{D}_{j}\mathbf{Q}_k,\ \sum_{k=1}^{N}\mathbf{\Lambda}_k\mathbf{E}_{zj}\geq \mathbf{E}_j-\mathbf{D}_{j}\mathbf{\hat{y}}
    \end{equation}
    where \(\mathbf{\Lambda}_k\) is some matrix with nonnegative entries, \(\sum_{k=1}^{N} \mathbf{Q}_k=\mathbf{P}_i\).
\end{lemma}
